# Supplementary material for: Reliable Geofence Activation with Sparse and Sporadic Location Measurements: Extended Version
Source: arXiv:2204.00714 source file (2022-04-01)
Supplement: Supplementary file 1 [file 07-appendix.tex]

\appendix
\section{Appendix}
\label{sec:appendix}

\subsection{Additional Data Statistics}

Figure~\ref{fig:lambda-histogram} show the histogram of $\lambda$ per minute for 1000 random trajectories. As $\lambda$ indicates the mean number of measurements over some unit time, this shows that there is often a small number of measurements every minute. The mode of this distribution of $\lambda$'s occurs at 0.04, which corresponds to one measurement every 25 minutes.

\begin{figure}[h]
\centering
\includegraphics[width=.9\linewidth]{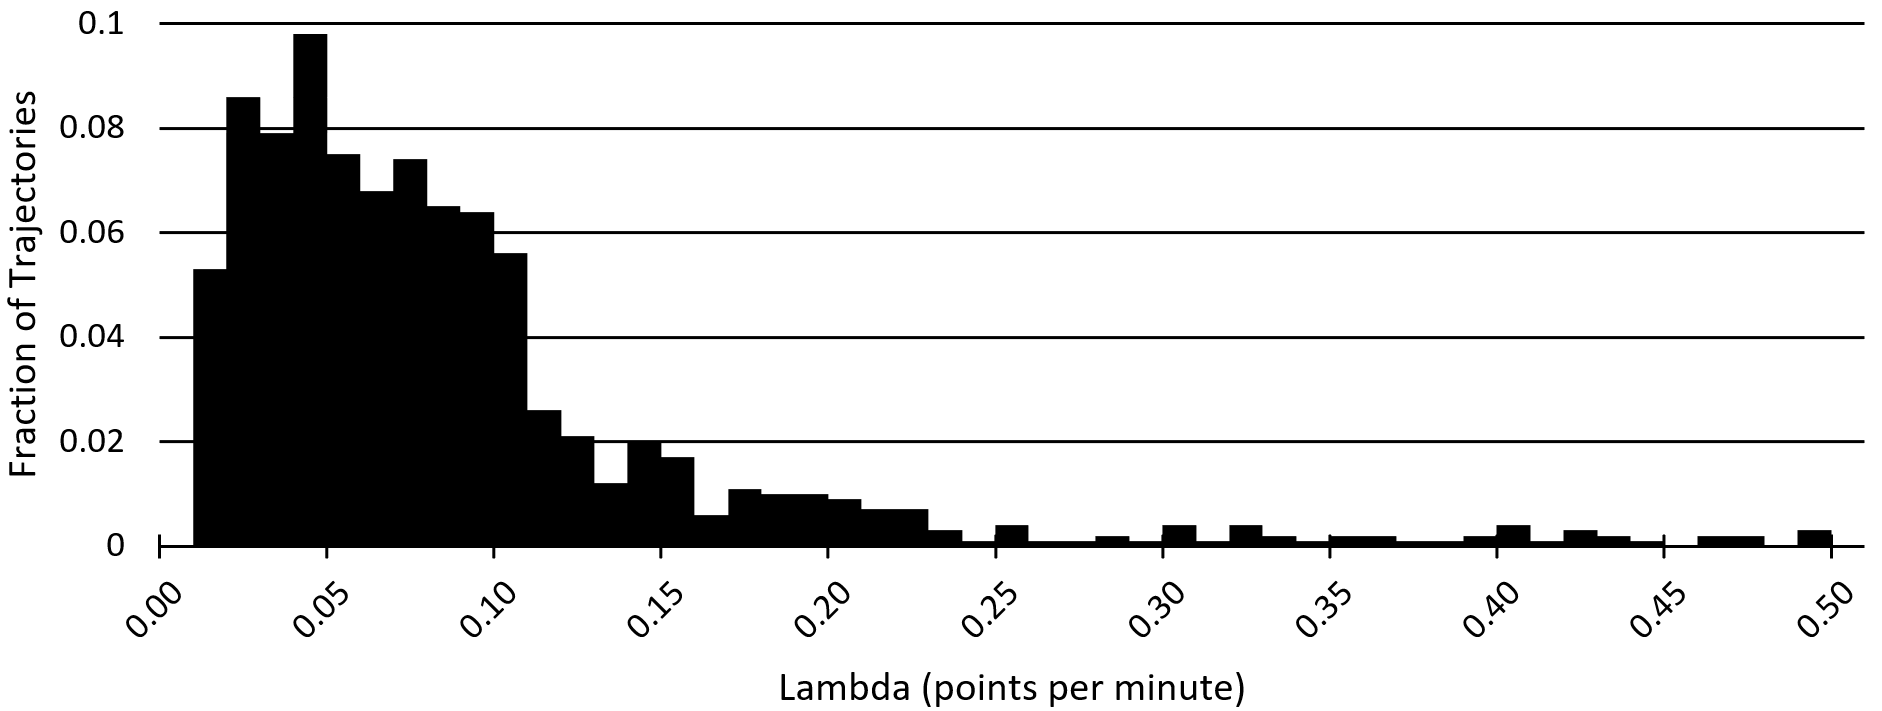}
\caption{Histograms of $\lambda$ for 1000 random trajectories.\label{fig:lambda-histogram}}
\end{figure}

\subsection{Additional Experimental Results}

Figure~\ref{fig:grid} shows an example of a grid of geofences being used for the experiments. The last data point of the training part of a trajectory is at the center of the grid. Each trajectory has its own grid of geofences.

\begin{figure}[h]
\centering
\includegraphics[width=.6\linewidth]{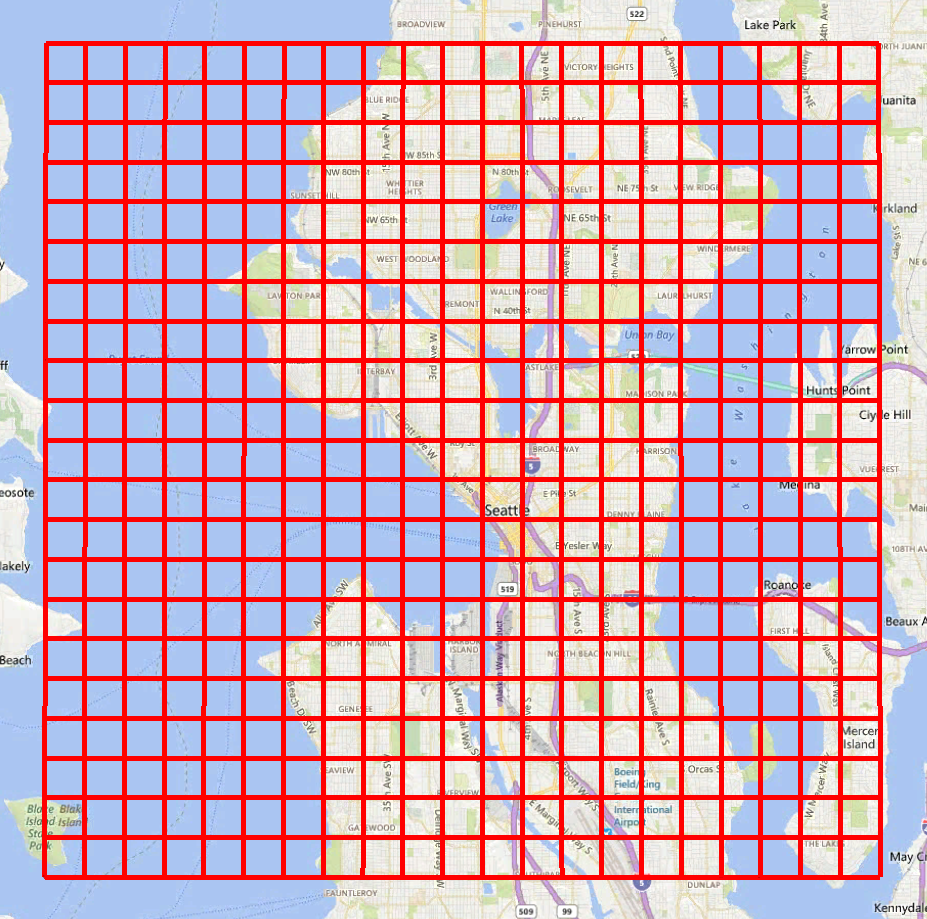}
\caption{An example of a grid of geofences being used for the experiments. Each cell is 1 km on a side.\label{fig:grid}}
\end{figure}

Figure~\ref{fig:vary_measurement_std_noise_added_before_training} show the realized values when the measurements is perturbed by adding Gaussian noises with standard deviation $\sigma_m$ to the measurements before providing the measurements to the prediction methods.

\begin{figure}[H]
\centering
\begin{subfigure}{.5\linewidth}
  \centering
  \includegraphics[width=\textwidth]{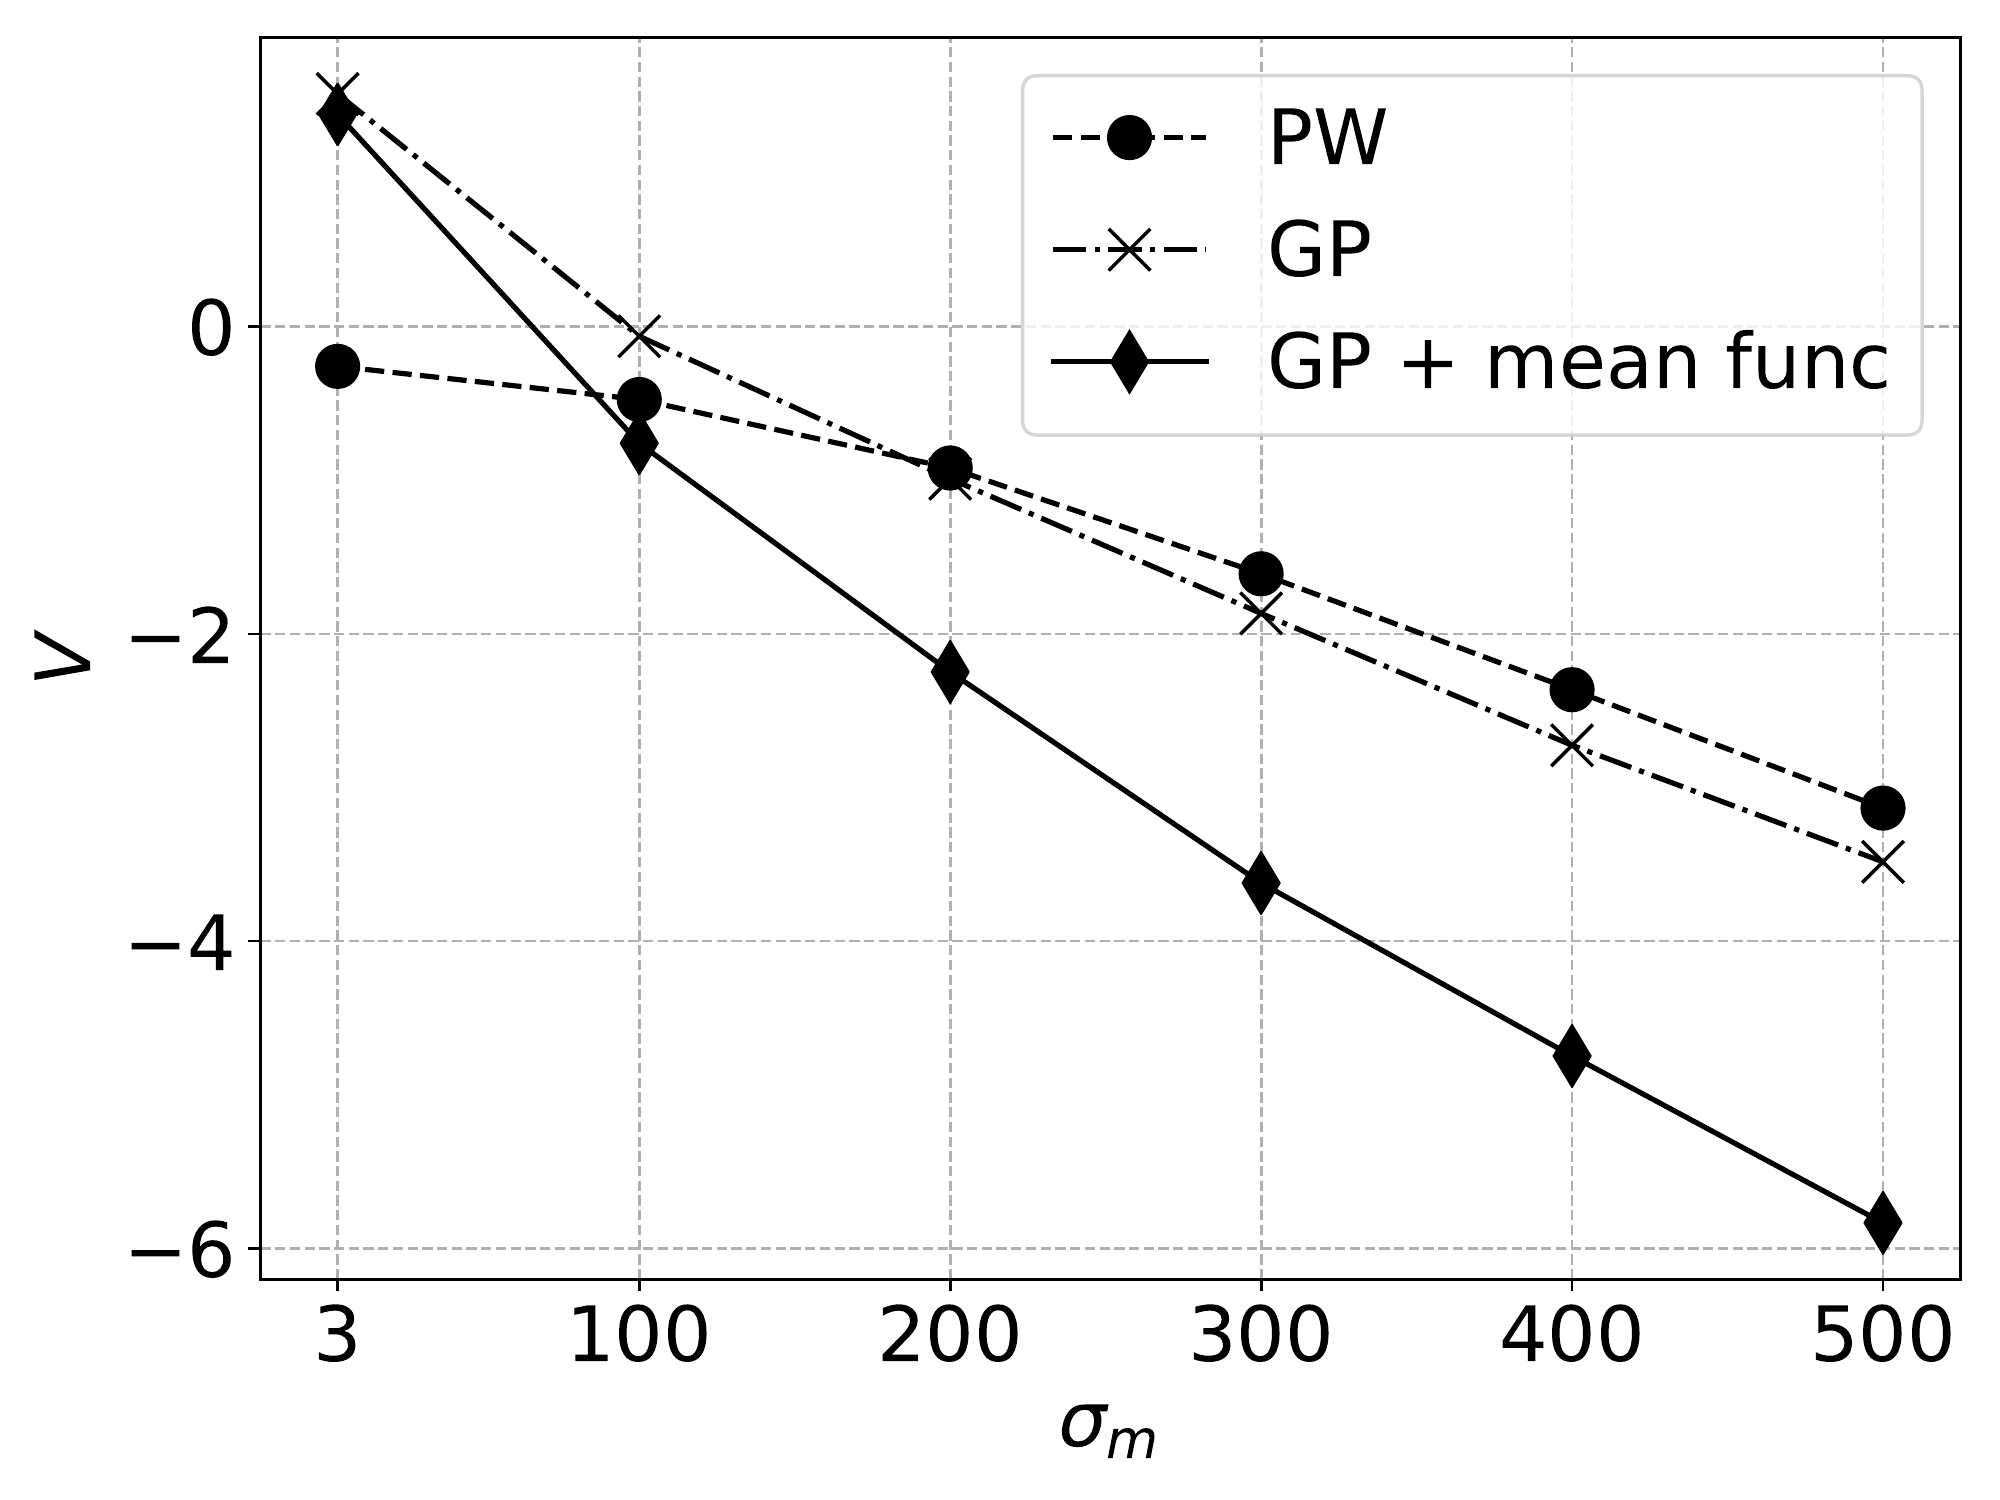}
  \caption{Advertising}
  \label{fig:vary_measurement_std_noise_added_advertising}
\end{subfigure}%
\begin{subfigure}{.5\linewidth}
  \centering
  \includegraphics[width=\textwidth]{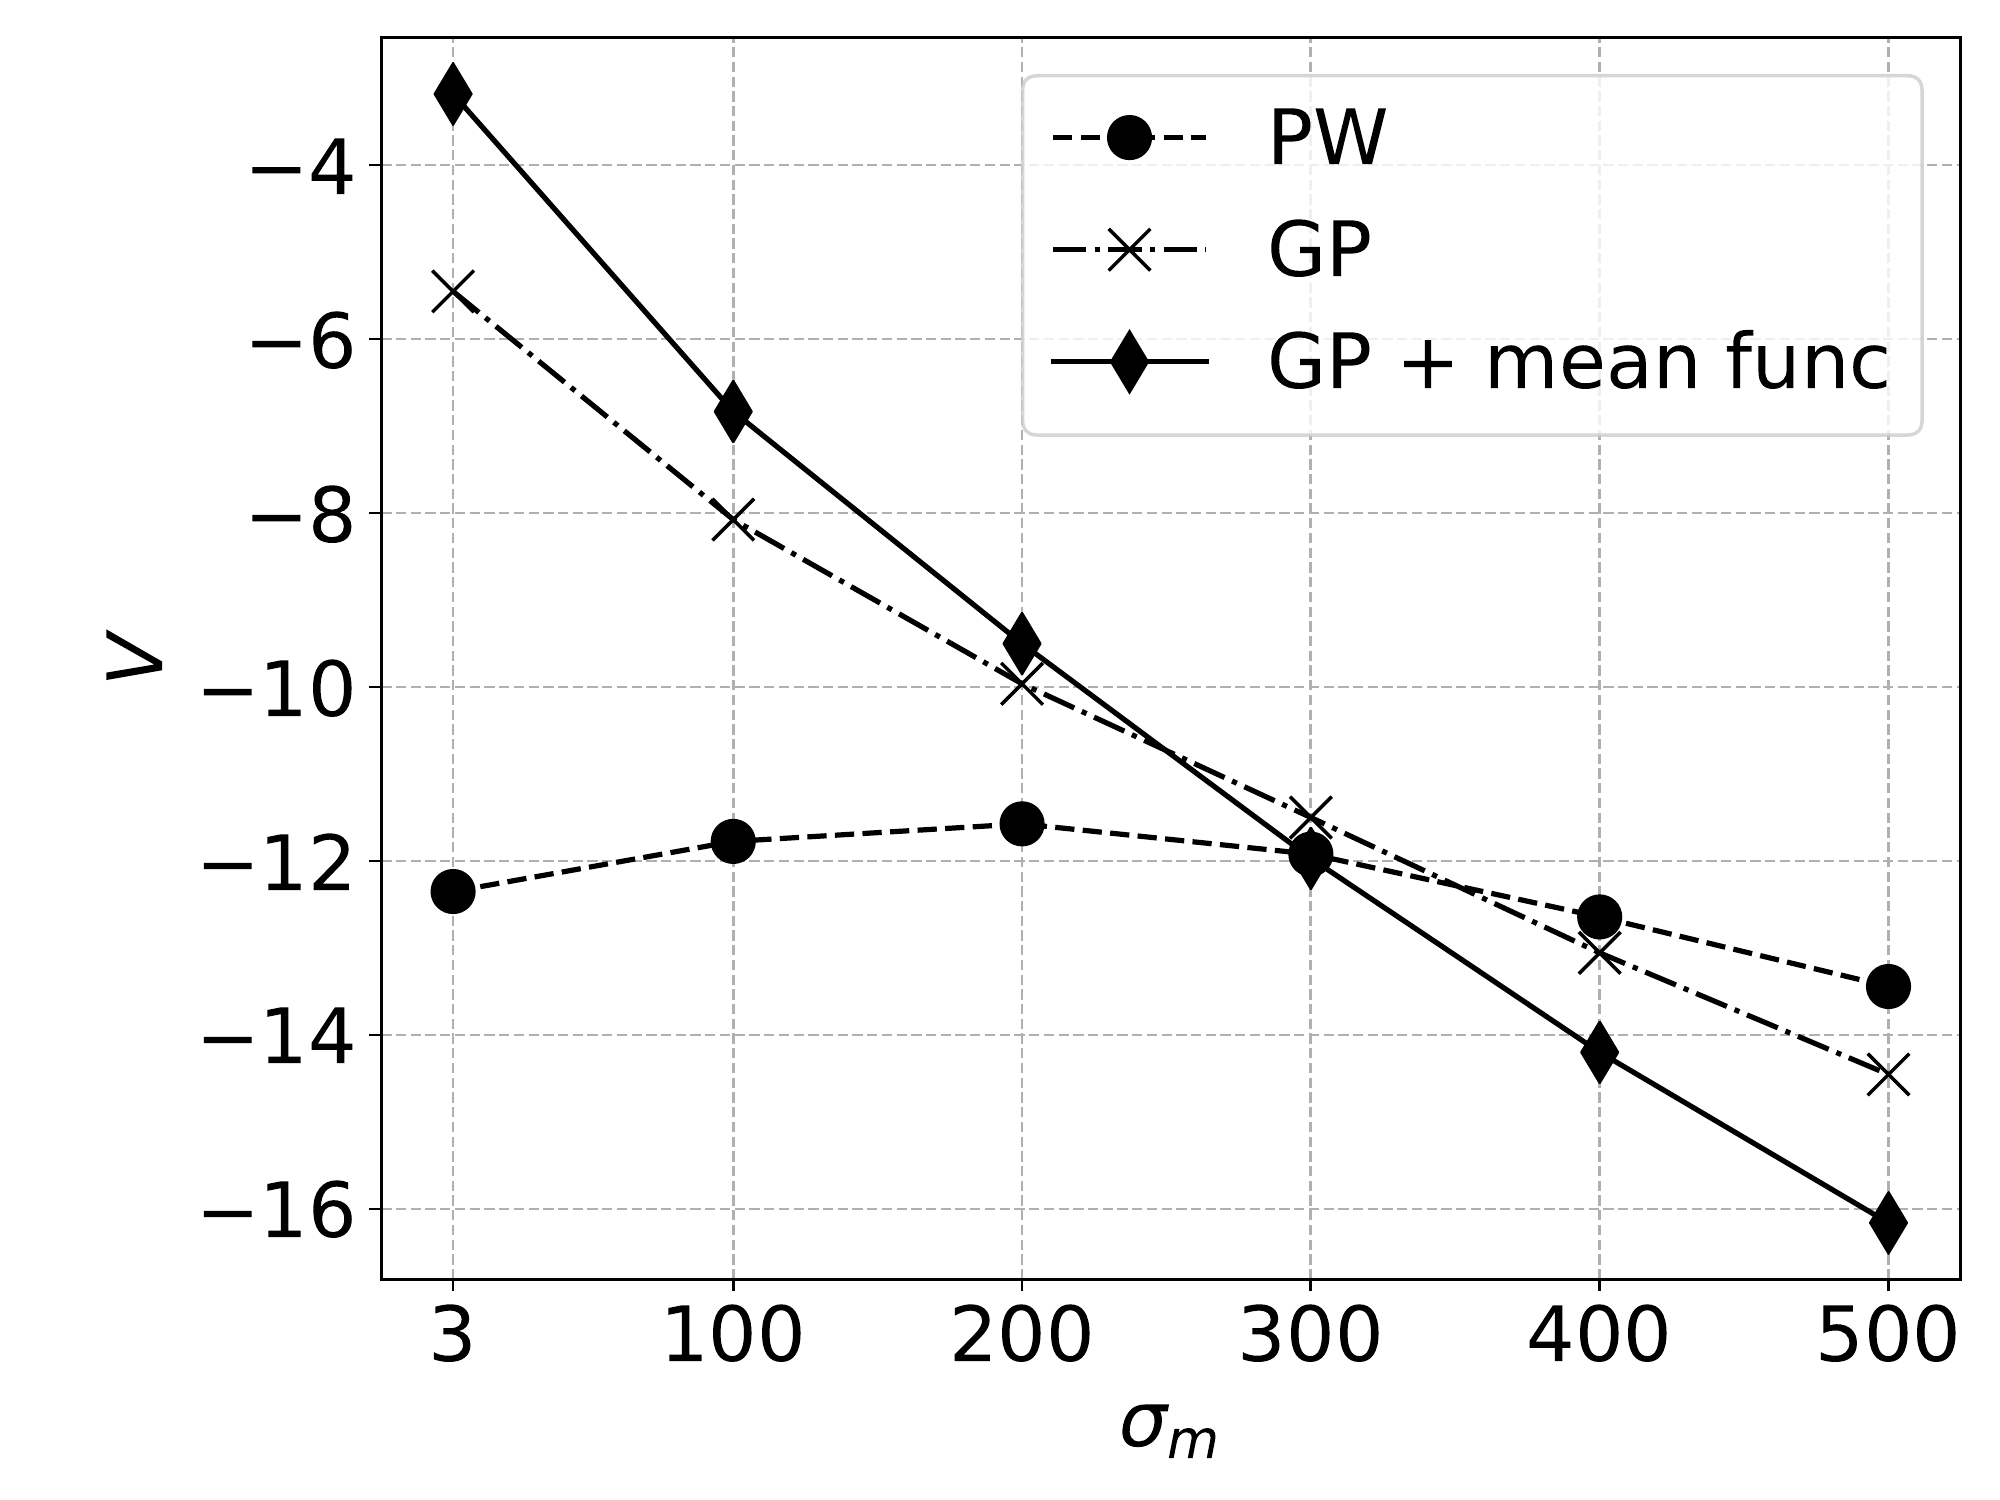}
  \caption{Alert-zone}
  \label{fig:vary_measurement_std_noise_added_alertzone}
\end{subfigure}
\caption{The realized values when varying measurement standard deviation $\sigma_m$ (in meters) with noises added before training}
\label{fig:vary_measurement_std_noise_added_before_training}
\end{figure}
